# Supplementary material for: Search for the direct production of charginos, neutralinos and staus in final states with at least two hadronically decaying taus and missing transverse momentum in $pp$ collisions at $\sqrt{s}$ = 8 TeV with the ATLAS detector
Source: arXiv:1407.0350 source file (2014-10-22)
Supplement: Supplementary file 1 [file Appendix.tex]

%!TEX root = DGSlepton2Lep.tex

\section*{Additional Material}

%%% Figure 10 %%%
\begin{figure}[!htbp]
\begin{center}
    \raisebox{0.33\textwidth}{(a)}\includegraphics[width=0.43\textwidth]{figaux_10a}
    \raisebox{0.33\textwidth}{(b)}\includegraphics[width=0.43\textwidth]{figaux_10b}
    \raisebox{0.33\textwidth}{(c)}\includegraphics[width=0.43\textwidth]{figaux_10c}
    \raisebox{0.33\textwidth}{(d)}\includegraphics[width=0.43\textwidth]{figaux_10d}
\caption{Signal regions contributing to the exclusion limit in the plane of 
(a) slepton mass and the lightest neutralino mass for combined right-handed selectrons and smuons,
(b) slepton mass and the lightest neutralino mass for combined left-handed selectrons and smuons,
(c) slepton mass and the lightest neutralino mass for combined left-handed and right-handed selectrons and smuons, and
(d) chargino mass and the lightest neutralino mass.
The different colors show which signal region, \SRmtta\ or \SRmttb, has the highest expected
sensitivity at a given mass point.
\label{regions_exclusion1}}
\end{center}
\end{figure}
%%% Figure 10 %%%

%%% Figure 11 %%%
\begin{figure}[!htbp]
\begin{center}
   \includegraphics[width=0.45\textwidth]{figaux_11}
\caption{Signal regions contributing to the exclusion limit in the
$m_{\neutralino{1}}$--$m_{\chargino{1}}$ plane.
The different colors show which signal region, \SRWWa, \SRWWb\ or \SRWWc, has the highest expected
sensitivity at a given mass point.
\label{regions_exclusion2}}
\end{center}
\end{figure}
%%% Figure 11 %%%

%%% Figure 12 %%%
\begin{figure}\centering
	\raisebox{0.33\textwidth}{(a)}\includegraphics[width=0.45\textwidth]{figaux_12a}\hfil
	\raisebox{0.33\textwidth}{(b)}\includegraphics[width=0.45\textwidth]{figaux_12b}
	\caption{\label{fig:WWFinalCLS}
		Observed (a) and  expected (b)  \CLs\ values from SR-$WW$a--c
		for simplified models with bino-like \neutralino{1} and wino-like \chargino{1}
		in the $m_{\neutralino{1}}$--$m_{\chargino{1}}$ plane.}
\end{figure}
%%% Figure 12 %%%

%%% Figure 13 %%%
\begin{figure}[!htbp]
\begin{center}
   \includegraphics[width=0.43\textwidth]{figaux_13a}
   \includegraphics[width=0.43\textwidth]{figaux_13b}
\caption{ 95\% exclusion limit for the mode  with intermediary sleptons 
in the plane with the chargino mass and the lightest neutralino mass.
(Left) The numbers in the plot quote the 95\% CL excluded limits on the model cross section in pb.
(Right) The number in the plot quote the \CLs\ value at a given mass point.
\label{exclusion_modeC_aux}}
\end{center}
\end{figure}
%%% Figure 13 %%%

%%% Figure 14 %%%
\begin{figure}[!htbp]
\begin{center}
   \includegraphics[width=0.43\textwidth]{figaux_14a}
   \includegraphics[width=0.43\textwidth]{figaux_14b}
\caption{ 95\% exclusion limit for combined right-handed selectrons and smuons.
(Left) The numbers in the plot quote the 95\% CL excluded limits on the model cross section in fb.
(Right) The number in the plot quote the \CLs\ value at a given mass point.
\label{exclusion_rhslep_aux}}
\end{center}
\end{figure}
%%% Figure 14 %%%

%%% Figure 15 %%%
\begin{figure}[!htbp]
\begin{center}
   \includegraphics[width=0.43\textwidth]{figaux_15a}
   \includegraphics[width=0.43\textwidth]{figaux_15b}
\caption{ 95\% exclusion limit for combined left-handed selectrons and smuons.
(Left) The numbers in the plot quote the 95\% CL excluded limits on the model cross section in fb.
(Right) The number in the plot quote the \CLs\ value at a given mass point.
\label{exclusion_lhslep_aux}}
\end{center}
\end{figure}
%%% Figure 15 %%%

%%% Figure 16 %%%
\begin{figure}[!htbp]
\begin{center}
   \includegraphics[width=0.43\textwidth]{figaux_16a}
   \includegraphics[width=0.43\textwidth]{figaux_16b}
\caption{ 95\% exclusion limit for combined right-handed and left-handed selectrons and smuons.
(Left) The numbers in the plot quote the 95\% CL excluded limits on the model cross section in fb.
(Right) The number in the plot quote the \CLs\ value at a given mass point.
\label{exclusion_rhlhslep_aux}}
\end{center}
\end{figure}
%%% Figure 16 %%%

%%% Table 6 %%%
\begin{table}[htbp]
\small
\begin{center}
\begin{tabular}{l|rr|rr}
\hline
$(m_{\SL},m_{\NONE})$ & \multicolumn{2}{c|}{$(191,90)\GeV$} & \multicolumn{2}{c}{$(250,10)\GeV$} \\
\hline
Lepton flavour & \multicolumn{1}{c}{\ee} & \multicolumn{1}{c|}{\mumu}
               & \multicolumn{1}{c}{\ee} & \multicolumn{1}{c}{\mumu} \\
\hline
Trigger    & 150\phantom{.0} & 159\phantom{.0} & 55\phantom{.0} & 50\phantom{.0} \\
$Z$ veto   & 139\phantom{.0} & 148\phantom{.0} & 54\phantom{.0} & 49\phantom{.0} \\
Jet veto   &  58\phantom{.0} &  62\phantom{.0} & 20\phantom{.0} & 20\phantom{.0} \\
\METrel\   &  45\phantom{.0} &  50\phantom{.0} & 17\phantom{.0} & 17\phantom{.0} \\
\hline
\SRmtta\   &  21.6           &  21.6           & 12.2           & 12.5 \\
\SRmttb\   &  12.3           &  12.0           & 10.5           & 11.2 \\
\hline
\end{tabular}
\caption{%
Expected numbers of signal events after each step of the event selection
for slepton-pair production benchmark model points,
$(m_{\SL},m_{\NONE})=(191,90)\GeV$ and $(250,10)\GeV$,
with common left- and right-handed slepton masses.
A total of 5000 events are generated in each sample.
The numbers are scaled to correspond to an integrated luminosity of 20.3\,\ifb.
\label{tlb:cutflow_mt2_SLep}
}
\end{center}
\end{table}
%%% Table 6 %%%

%%% Table 7 %%%
\begin{table}[htbp]
\small
\begin{center}
\begin{tabular}{l|rrr|rrr}
\hline
$(m_{\CONEPM},m_{\NONE})$ & \multicolumn{3}{c|}{$(350,0)\GeV$} & \multicolumn{3}{c}{$(425,75)\GeV$} \\
\hline
Lepton flavour & \multicolumn{1}{c}{\ee} & \multicolumn{1}{c}{\mumu} & \multicolumn{1}{c|}{\emuOS}
               & \multicolumn{1}{c}{\ee} & \multicolumn{1}{c}{\mumu} & \multicolumn{1}{c}{\emuOS} \\
\hline
Trigger   & 52\phantom{.0} & 48\phantom{.0} & 79\phantom{.0} & 20\phantom{.0} & 20\phantom{.0} & 31\phantom{.0} \\
$Z$ veto  & 48\phantom{.0} & 45\phantom{.0} & 74\phantom{.0} & 19\phantom{.0} & 19\phantom{.0} & 29\phantom{.0} \\
Jet veto  & 20\phantom{.0} & 19\phantom{.0} & 30\phantom{.0} &  7\phantom{.0} &  7\phantom{.0} & 11\phantom{.0} \\
\METrel\  & 17\phantom{.0} & 17\phantom{.0} & 25\phantom{.0} &  6\phantom{.0} &  6\phantom{.0} &  9\phantom{.0} \\ 
\hline
\SRmtta\  & 11.7           & 10.5           & 16.6           &  4.3           &  4.4           &  6.7 \\
\SRmttb\  &  9.5           &  8.7           & 14.0           &  3.7           &  3.8           &  1.1 \\
\hline
\end{tabular}
\caption{%
Expected numbers of signal events after each step of the event selection
for chargino-pair production with intermediary slepton benchmark model points,
$(m_{\CONEPM},m_{\NONE})=(350,0)\GeV$ and $(425,75)\GeV$.
A total of 40000 events are generated in each sample.
The numbers are scaled to correspond to an integrated luminosity of 20.3\,\ifb.
\label{tlb:cutflow_mt2_modeC}
}
\end{center}
\end{table}
%%% Table 7 %%%

%%% Table 8 %%%
\begin{table}
\begin{center}
\begin{tabular}{l|r|r|r|r}
\hline
Signal model          & \multicolumn{1}{c|}{S1} & \multicolumn{1}{c|}{S2} 
                      & \multicolumn{1}{c|}{S3} & \multicolumn{1}{c}{GMSB} \\
\hline
No Cuts               & 11003\phantom{.0} & 3393\phantom{.0} & 749\phantom{.0} & 10239\phantom{.0} \\
All cleaning          & 10691\phantom{.0} & 3299\phantom{.0} & 732\phantom{.0} & 10066\phantom{.0} \\
Two signal leptons    &  3178\phantom{.0} & 1060\phantom{.0} & 261\phantom{.0} &  3960\phantom{.0} \\
Trigger               &  2559\phantom{.0} &  872\phantom{.0} & 214\phantom{.0} &  3097\phantom{.0} \\
\emu\                 &   861\phantom{.0} &  296\phantom{.0} &  71\phantom{.0} &   661\phantom{.0} \\
Jet veto              &   443\phantom{.0} &  139\phantom{.0} &  31\phantom{.0} &   241\phantom{.0} \\
$(\pT^{\ell1},\pT^{\ell2}>(35,20)\GeV$
                      &   310\phantom{.0} &  103\phantom{.0} &  25\phantom{.0} &   167\phantom{.0} \\
\hline
\SRWWa               & $31.5$  &         &         & $18.2$\\
\SRWWb               &         & $8.2$   &         & $4.3$\\
\SRWWc               &         &         & $3.3$   &       \\
\hline
\end{tabular}
\end{center}
\caption{%
Expected numbers of signal events after each step of the event selection
for benchmark model points in the \SRWW.
The numbers are scaled to correspond to an integrated luminosity of 20.3\,\ifb.
The signal models S1, S2 and S3 are chargino-pair production with wino-like
\chargino{1} and bino-like \neutralino{1} with
$(m_{\chargino{1}},m_{\neutralino{1}})=(100,0)\GeV$, $(140,20)\GeV$ and $(200,0)\GeV$,
respectively.
The GMSB model has $m_{\chargino{1}}=110\GeV$, $m_{\neutralino{1}}=113\GeV$, and
the LSP is a massless gravitino.}
\label{tab:CutFlowSRWW}
\end{table}
%%% Table 8 %%%
